# Supplementary material for: Off-Dynamics Inverse Reinforcement Learning from Hetero-Domain
Source: arXiv:2110.11443 source file (2021-10-21)
Supplement: Supplementary file 1 [file 8-appendix.tex]

\section{JUSTIFICATION OF ODIRL}
\url{https://anonymous.4open.science/r/ODIRL-BD1D/}
